# Supplementary material for: Validity of Stokes-Einstein Relation in Soft Colloids up to the Glass Transition
Source: arXiv:1508.07241 source file (2015-08-31)
Supplement: Supplementary file 1 [file Supplementary-Material.pdf]

# Supplementary Material for: Validity of Stokes-Einstein Relation in Soft Colloids up to the Glass Transition

Sudipta Gupta,[1,2] Jörg Stellbrink,[1] Emanuela Zaccarelli,[3] Christos N. Likos,[4]
Manuel Camargo,[5] Peter Holmqvist,[6] Jürgen Allgaier,[1] Lutz Willner,[1] and Dieter Richter[1]

[1] *JCNS-1 and ICS-1, Forschungszentrum Jülich, Leo-Brandt-Straße, 52425 Jülich, Germany*
[2] *JCNS-SNS, Oak Ridge National Laboratory, Bethel Valley Road, TN-37831 Oak Ridge, USA*
[3] *CNR-ISC and Dipartimento di Fisica, Universitá di Roma La Sapienza Piazzale A. Moro 2, I-00185, Roma, Italy*
[4] *Faculty of Physics, University of Vienna, Boltzmanngasse 5, A-1090 Vienna, Austria*
[5] *Centro de Investigaciones en Ciencias Básicas y Aplicadas, Universidad Antonio Nariño, Km 18 via Cali-Jamundí, 760030 Santiago de Cali, Colombia*
[6] *Division of Physical Chemistry, Lund University, 22100 Lund, Sweden*

(Dated: August 27, 2015)

## Sample preparation

All diblock copolymer solutions, from dilute to close to the overlap volume fraction $\phi^*$, were prepared in the same way by mixing the desired amounts of polymer powder and solvent ($D_2O$) in sterilized vials. Correct component amounts were weighted using a BP211D Sartorius balance, with an accuracy of 0.01 mg. Previously to mixing, the solvent was filtered two times using Anotop membrane filters of 20 nm pore size and the sample containers were filled with Argon in order to prevent possible degradation of the PEO chain due to oxidation. Dilute solutions mix spontaneously and were then put into electronic shaker to homogenize them at 20°C overnight. Whereas the more concentrated solutions were heated up to 40°C several times, maximum for five hours, with continuous shaking. Extremely viscous solutions close to $\phi^*$ where homogenized using as sequence of vortex mixing and centrifugation at 40°C several times. Before performing any experiments, all samples were found to be optically transparent and homogeneous. Polymer degradation was checked afterwards by SEC measurements of the molecular weight distribution. Fully homogenized samples were finally filtered into the measurement cells for PFG-NMR and DLS using Anotop membrane filter of 200 nm pore size. For samples with $N_{\rm agg} = 500$ and the highest concentrations, filtration was not applicable due to the high viscosity and therefore the samples were directly transferred into the measurement cells using sterilized pipettes. In addition, to avoid dust contamination crucial for DLS all measurement cells were rinsed several hours using an acetone fountain. In addition, before measurements samples were allowed to equilibrate for 1-5 days. It should be noted that to maintain consistency for all the experiments (PFG-NMR, DLS and rheology) we have always used $D_2O$ as the solvent.

## DLS experiment and modeling

Corresponding SLS/DLS measurements were performed on a standard light scattering setup with ALV-125 compact goniometer and ALV5000E correlator covering a range of scattering angles $20^\circ \leq \theta \leq 150^\circ$ and corresponding $Q$-range $6\times10^6 \leq Q \leq 3.1\times10^7\,\mathrm{m}^{-1}$. Two different lasers were used ($\mathrm{Ar}^+$ with $\lambda = 514.5$ nm, and He-Ne with $\lambda = 632.8$ nm), depending on the scattering intensity of the sample. Temperature control of $20 \pm 0.01$°C was set by a circulating fluid bath thermostat (Julabo, Germany). For all samples, measurement times were adjusted to the slowest observed relaxation processes which means for samples close to $\phi^*$ measurement times of up to 12 hours. The influence of laser stability was also carefully checked.

For dynamic light scattering (DLS) our data analysis of the experimental intensity autocorrelation function (IACF) $g_e^{(2)}(Q,t)$ was based on the inverse-Laplace transformation by using CONTIN algorithm developed by Provencher [1] i.e.

$$g_e^{(1)}(Q,t) = \frac{1}{2\pi}\int_0^\infty d\Gamma G(\Gamma)\exp\left(-\Gamma t\right), \qquad (1)$$

where $G(\Gamma)$ is the distribution of relaxations frequency $\Gamma$. We use the CONTIN algorithm as provided by the ALV-software with up to 250 grid points, variation of the used frequency window on the results was tested.

For diffusive motion holds $\Gamma = 1/t_s = DQ^2$, where $D$ and $t_s$ are the diffusion coefficient of the scattering particles and the relaxation time, respectively. DLS usually measures the collective diffusion coefficient $D_{\rm coll}$ from which the

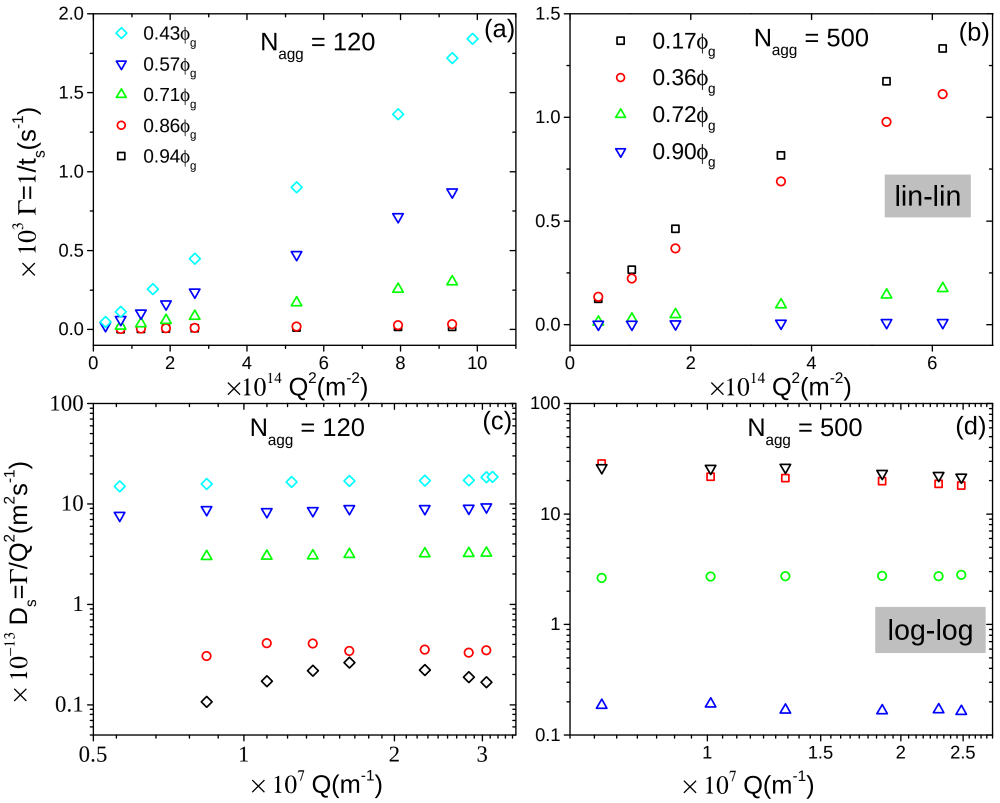


FIG. S1: The diffusive nature of the relaxation time $t_s = 1/\Gamma$, which corresponds to the self diffusion coefficient $D_s$ as a function of the square of the scattering wavevector $Q$ for $N_{\rm agg} = 120$ [(a) and (c)] and $N_{\rm agg} = 500$ [(b) and (d) ]. Different volume fractions $\phi$ are expressed in the legend in terms of the volume fraction $\phi_g$ at the glass transition. The upper plots are displayed in linear scale whereas the lower ones are in logarithmic scale.

self diffusion coefficient $D_s$ can be obtained by extrapolation to infinite dilution. We have to note that $D_s$ can be directly measured by PFG-MNR. Both diffusion coefficients show a strong concentration dependence and only at infinite dilution $D_{\rm coll} = D_s$ holds. With increasing concentration, $D_{\rm coll}$ is increasing due to hydrodynamic and direct interactions whereas $D_s$ is slowed down. At finite concentration, DLS can only measure $D_s$ in case of scattering strength polydispersity, which is given for star polymers and star-like micelles due to functionality or aggregation number polydispersity (see also section mixing below). Therefore, we observed with increasing concentration a splitting of the one peak in $G(\Gamma)$ into a bimodal distribution reflecting $D_{\rm coll}$ and $D_s$, which were separating more and more until finally the difference is several orders of magnitude. The identification of the slower mode as self diffusion is unambiguously confirmed by comparison with PFG-NMR results, as shown in Figure 4 of the main manuscript.

Figure S1 illustrates the variation in relaxation time $t_s$ as a function of $Q^2$ for $N_{\rm agg} = 120$ and $N_{\rm agg} = 500$, as well as $D_s$ as a function of $Q$ for different volume fractions $\phi$, the latter being expressed in terms of the volume fraction at the glass transition, $\phi_g$. It clearly highlights the diffusive nature ($\sim Q^{-2}$) of the relaxation time. It should be noted that we have repeated each measurement between 1 to 5 days after sample preparation and no effect of aging was visible below and around the overlap volume fraction $\phi^*$.

### Rheology experiment and modeling

To investigate the viscoelastic flow behavior of the samples we performed rheological experiments using both stress-controlled (AR-G2) rheometer (Rheometric Scientific Company) and capillary viscometer. We used cone-plate geometry made of stainless steel of cone diameter $20 - 50$ mm at a cone angle $0.01 - 0.04$ rad, depending on the concentration of the samples. Temperature control of $20 \pm 0.01°$C was set via a Peltier plate and was cooled by a circulating fluid bath thermostat (Julabo, Germany). From rheology we measured the change in viscosity $\eta$ as a function of shear rate $\dot\gamma$ by direct flow curves, covering the range $10^{-3} < \dot\gamma < 3 \times 10^3$ s$^{-1}$. By repeating each

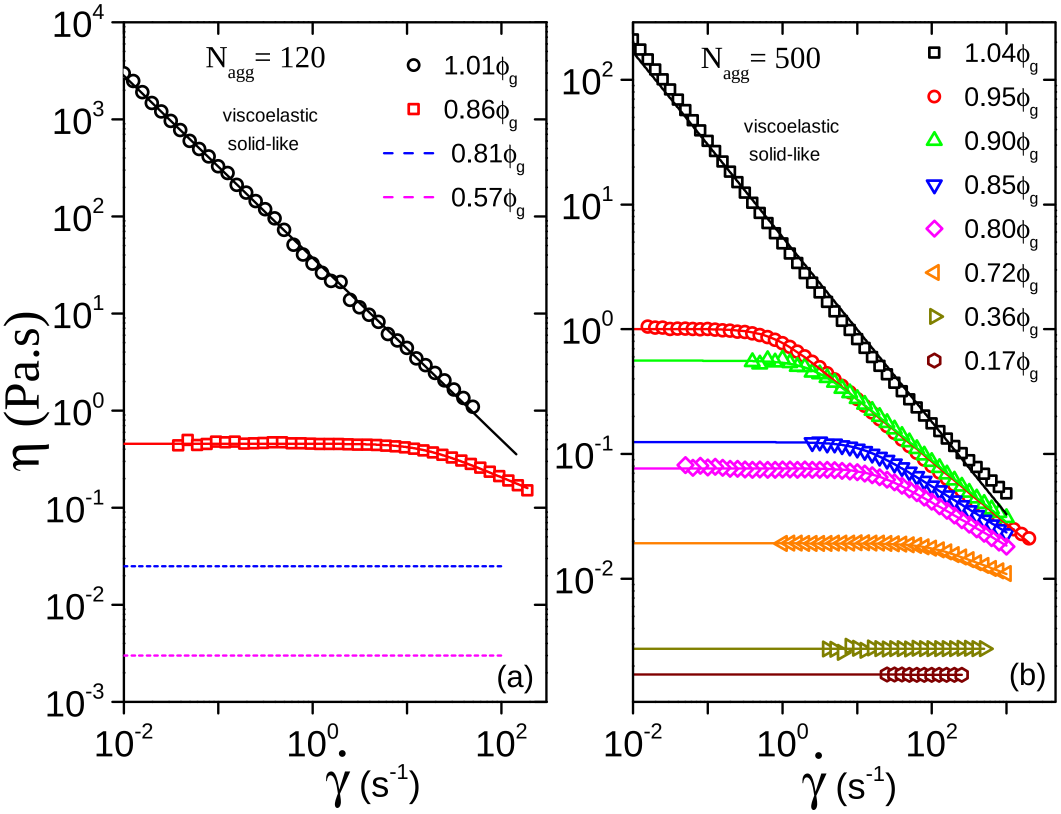


FIG. S2: Flow curves for (a) $N_{\rm agg} = 120$ and (b) $N_{\rm agg} = 500$ at different volume fractions $\phi$, indicated in units of the glass volume fraction $\phi_g$. For $N_{\rm agg} = 120$ and volume fractions below $0.86\phi_g$, viscosity was determined by capillary viscometry as illustrated by the dashed lines. Solid lines indicates fitting to Eq. (2). For both systems, the highest concentrations above $\phi_g$ showed viscoelastic solid-like behavior.

measurement we have checked the data reproducibility. To ensure steady state of the sheared sample, we followed a strict protocol as described by Petekidis *et al.* [2]. We measured each data point (shear rate) at 300 s intervals along with increase in measurement time as the shear rate decreases. We performed a 10 s pre-shear protocol, followed by a 10 s measurement, for all $\dot{\gamma} > 1$ s$^{-1}$. A pre-shear for 100 s, followed by a 100 s measurement time were employed for $10^{-2} < \dot{\gamma} \leq 1$ s$^{-1}$. Finally a pre-shear of 1000 s with a 1000 s measurement time were performed for all $\dot{\gamma} \leq 10^{-2}$ s$^{-1}$.

Figure S2 illustrates the flow curves, i.e. viscosity $\eta$ vs. shear rate $\dot{\gamma}$ curves, for $N_{\rm agg} = 120$ and $N_{\rm agg} = 500$ at different volume fractions. To yield the zero-shear viscosity $\eta_0$ and to investigate the shear rate dependent viscosity (*shear thinning*), the flow curves were fitted to the Carreau equation given by [3]:

$$\frac{\eta(\dot{\gamma}) - \eta_\infty}{\eta_0 - \eta_\infty} = \frac{1}{[1 + (\dot{\gamma}/\dot{\gamma}_c)^a]^{\frac{1-b}{a}}}, \tag{2}$$

where $\eta_\infty$ denotes the high shear-rate Newtonian limit of viscosity. Frequently, the high shear rate region is not observed and thus $\eta_\infty$ was set to zero in Eq. (2). The quantity $\dot{\gamma}_c$ indicates the onset of the shear thinning and has the dimensions of s$^{-1}$; the power law exponent, $(1 - b)$, describes the dependence of the viscosity on shear rate in the shear thinning region. For our samples, the value of $(1 - b)$ lies between 0.2 and 0.76 at intermediate concentration for $\phi < \phi^*$. It is to be noted that for dilute concentration, $(1 - b) = 0$ gives the Newtonian plateau with zero-shear viscosity $\eta_0$. The additional dimensionless parameter $a$ represents the width of the transition region between the constant Newtonian plateau observed at low shear rates and the asymptotic power law decrease of the viscosity found at high shear rates. Value of $a = 2$ is kept constant.

All viscosities below $0.86\phi_g$ for $N_{\rm agg} = 120$ in Fig. S2 were determined by capillary viscometry as illustrated by the dashed lines. For both systems, the highest concentrations above $\phi_g$ show viscoelastic, solid-like behavior, where the corresponding zero shear viscosity is ill-defined. This behavior was also verified from oscillatory measurements using strain-controlled ARES-G2 rheometer, where the storage modulus $G'$ was greater than the loss modulus $G''$. We followed a pre-shear protocol of 200 s interval of oscillatory shearing at $\omega = 1$ rad/s with strain amplitude $\gamma_0 = 100\%$,

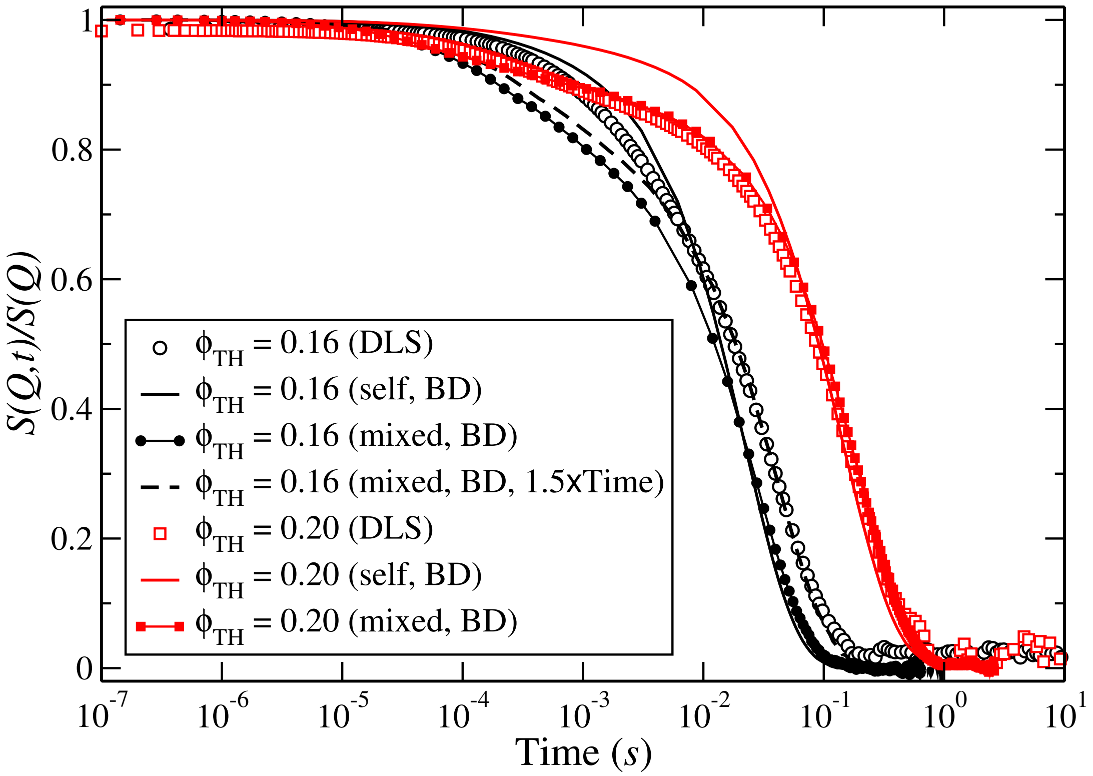


FIG. S3: Normalized dynamic structure factor or density autocorrelation functions at $Q\sigma_{\rm int} \simeq 1.68$ for $N_{\rm agg} = 500$ and $\phi_{\rm TH} = 0.16$ and 0.20, as indicated. The dashed lines represents the self correlation functions calculated from BD simulation. The solid lines are linear combinations of 70% self and 30% collective density correlations from BD for both densities. For the low density curve, a small mismatch is observed on the timescale, quantified by the arbitrary multiplication by a factor 1.5 in time, which could result from the uncertainties on packing fraction. For the high density the agreement is achieved without any other adjustment.

which placed the system in an initially homogeneous reproducible state, followed by a frequency sweep experiment over $100 \leq \omega \leq 0.1$ rad/s with $\gamma_0 \leq 1\%$. Each data point was measured for 10 s for $\omega > 1$ rad/s, and 100 s for $\omega \leq 1$ rad/s. To avoid sample evaporation for long measurement times, we sealed the sample with a layer of dodecane around the cone and plate of the rheometer. It is important to mention that no aging behavior was visible below and around the overlap volume fraction $\phi^*$. This was verified by varying the waiting time between the pre-shear protocol and the applied stain in steps between 100 s and 500 s, where all the data sets for $G'$ and $G''$ overlapped.

### Mixing

It is well-known that DLS measures typically collective relaxation processes arising from coherent scattering, but due to size and functionality polydispersity, also self-relaxation processes arising from incoherent scattering become observable [5, 6]. The agreement of diffusion coefficients obtained from DLS and PFG-NMR, as shown in Fig. 4 in the main manuscript, clearly identifies the slow mode as self-difusion. Indeed it can be seen in Fig. 2 of the main article (e.g., data for $\phi_{\rm TH} = 0.196$ for $N_{\rm agg} = 500$) that actually, the experimental curve is somehow intermediate between the self and collective correlators concerning the intermediate plateau value, indicating that a “mixing” of collective and self-correlators from BD simulation would be best suited to compare with the DLS data. This is shown in Figure S3, where the experimentally measured correlators are plotted for $N_{\rm agg} = 500$, $Q\sigma_{\rm int} \simeq 1.68$, and $\phi_{\rm TH} = 0.16$ and 0.20 and are compared to a “mixed” collective and self-correlators from BD simulations. Here we use a linear combination of 70% self and 30% collective density correlations from BD which perfectly superimposes on the experimental data for $\phi_{\rm TH} = 0.20$. For $\phi_{\rm TH} = 0.16$ a good agreement is also found. We notice that at this experimental volume fraction a small mismatch is present in the timescale, even for the pure correlators, that can be quantified by a small multiplicative factor on the time axis. This could result by experimental uncertainty e.g. on the value of the volume fraction. However, with such small adjustment, also at this density the data perfectly superimpose. However, we

could not find a general recipe for taking into account the mixing of self and collective contributions, which is found to depend on $N_{\rm agg}$ and slightly on $Q$, but crucially not on $\phi_{\rm TH}$. The detailed understanding of these issues are beyond the scope of the present paper.

[1] S. W. Provencher, Comp. Phys. Comm. **27**, 229 (1982); Comp. Phys. Comm. **27**, 213 (1982).
[2] G. Petekidis et al., J. Phys.: Condens. Matter, **16**, S3955 (2004).
[3] R. B. Bird, R. C. Armstrong and O. Hassager, *Dynamics of Polymeric Liquids*, Vol. 1, John Wiley and Sons, New York (1987).
[4] W. M. Macosko, *Rheology Principles, Measurements and Applications*, Wiley-VCH, New York (1994).
[5] R. Seghrouchni et al., Euro. Phys. Lett. **42**, 271 (1998).
[6] P. N. Pusey et al., J. Chem. Phys. **77**, 4270 (1982).
[7] D. Vlassopoulos et al., J. Phys.: Condens. Matter **13**, R855 (2001).
